# Supplementary material for: Redescription Model Mining
Source: arXiv:2107.04462 source file (2021-07-09)
Supplement: Supplementary file 1 [file XX_supplementary.tex]

The general procedure used when creating a single dataset is the same for all model classes.
Given \emph{model parameters} $\Theta$ and \emph{realisation parameters} $\Theta'$ we use a function generate\_tuples that can generate us a number $N$ of tuples given parameters $\theta=(\Theta, \Theta')$.
We assume that the parameters of a fit to $N$ of those tuples converges towards the \emph{model parameters} for a large $N$.
The \emph{realisation parameters} do not directly influence the model but are required to fix how exact the tuples are generated.
For a line generate a tuple (x,y) of points that lie along this line.
The parameters $\Theta$) fix slope and intercept. 
The realisation parameters $\Theta'$ indicate whether we e.g. sample x coordinates in $[1,2]$ or $[-10,-5)$ or how large the spread in the y direction around the line is.
Notice though that changing these realisation parameters do not change the parameters of a fit to the tuples when enough tuples are drawn.

%For the model to have that slope and intercept as $N \to \infty$ it doesn't matter 

To create a dataframe for redescription model mining pairs of parameters $\theta_i = (\Theta_i, \Theta_i')$ and randomly choose the number of tuples to be generated for those parameters.
We then draw tuples using the generate\_tuples function for all those pairs and stack them.
We indicate which model the points belong to through an additional nominal attribute called 'phenomenon'.
This already enables exceptional model mining but the discovered patterns are obvious and trivial as the subgroups are directly accessible through the 'phenomenon' attribute.

To increase the difficulty of the search we are including columns which make finding the implanted models harder.
This is necessary as we are not expecting phenomena being observable through only one indicative variable (in our case selecting 'phenomenon'=i).
%we hide the phenomena at depth $d$.
To that end, we introduce new binary columns $phenomenon_{i j}$, $j \in [0..d)$ which yield the set 'phenomenon'=i when intersected over $j$.
I.e. we are hiding the raw set of tuples corresponding to one model at depth $d$.
We firstly randomly draw pollution points $P$ ($|P| =n_{p} d$) from the set 'phenomenon'$\neq$ i without replacement.
This set is then split into $d$ disjoint sets $P_k$.
The new columns $phenomenon_{i j}$ are created by unifying the set 'phenomenon'==i with the sets $\{P_k | k\in[0..d) \land k \neq j\}$.
Now only a conjunction over $j$ of all the $phenomenon_{i j}$ columns will yield the not polluted tuples which correspond to the implanted model $i$.

Now that we can generate a single dataframe from parameters, we can use that to generate two dataframes with similar implanted models.
Simply use the generated $\theta_i$ to generate two datasets.
How we obtain the $\theta_i$ is model specific and discussed below.
%Given that we can (somehow) generate model and realisation parameters $\theta$. The exact way these are generated depends on the model but is not important for this point.
%Parameters
For out experiments we designate one set of parameters as the background parameters from which the majority of points are drawn.
This results in many models fitted to subgroups that will roughly follow the same distribution.
In addition we also implant 10 model parameters from which fewer tuples are generated.
We hide these implanted subgroups at a depth of $d=2$, chose the size of the background model to be a uniform random number between 10k and 100k for correlation models and between 1k and 10k for linear regression models. The implanted models subgroups sizes are chosen randomly between 5\% to 10\% of the background size.

\paragraph{Preprocessing for the housing datasets}
For both datasets we discarded extremely large houses (size $>$200), discarded observations with abnormal values and normalised the price by the corresponding standard deviation.
Interesting sidenote: It turns out we were able to approximately recover the exchange rate that way.
Finally we removed houses with a normalised price larger than 5.
Regarding the attributes, we have identified some translation errors for the Bejing dataset and tried to correct them.
We applied equal frequency binning with a number of 5 bins to numerical attributes.
We chose likelihood gain as exceptionality measure and Common Model Cooks similarity as similarity. To compensate for overly small subgroups, we multiplied the likelihood gain with the relative size to the power of $0.5$. We choose $\alpha_s=0.5$ and $\alpha_e=1.0$.
